# Supplementary material for: PC-Planner: Physics-Constrained Self-Supervised Learning for Robust Neural Motion Planning with Shape-Aware Distance Function
Source: arXiv:2410.12805 source file (2024-09-30)
Supplement: Supplementary file 1 [file 7_supp_figure.tex]

\input{figs/texs/adaptive_plan}

\input{figs/texs/turtlebot}

\input{figs/texs/ur5}

\input{figs/texs/plan_example}

\input{figs/texs/custom_arm}
